# Supplementary material for: Nonlinear optical effects in a nucleus
Source: arXiv:2008.12956 source file (2020-08-29)
Supplement: Supplementary file 1 [file Supplemental_Materials.pdf]

# Supplemental materials for "Nonlinear optical effects in a nucleus"

Tao Li[1] and Xu Wang[2,*]
[1]Beijing Computational Science Research Center, Beijing 100193, China
[2]Graduate School, China Academy of Engineering Physics, Beijing 100193, China
(Dated: August 29, 2020)

## I. HAMILTONIAN AND TIME-EVOLUTION OPERATORS

The total Hamiltonian of the deuteron in an electromagnetic field can be separated into a center-of-mass part and a relative-motion part. Since it is the dissociation process that is of interest, we will be focusing on the latter part, which has the following terms

$$H = \frac{\hat{\boldsymbol{p}}^2}{2\mu} + V_{pn} + V_L, \tag{S1}$$

where $\hat{\boldsymbol{p}}$ is the momentum operator for the relative motion, $\mu = M/2$ is the reduced mass with $M$ the mass of the proton (also approximately of the neutron), $V_{pn}$ is the (phenomenological) p-n potential, and $V_L$ is the interaction potential with the external light field. For convenience let us also define

$$H_0 = \frac{\hat{\boldsymbol{p}}^2}{2\mu} + V_{pn}; \tag{S2}$$

$$H_L = \frac{\hat{\boldsymbol{p}}^2}{2\mu} + V_L, \tag{S3}$$

both being part of the total Hamiltonian $H$.

In the so-called velocity gauge, the interaction potential $V_L$ is given as

$$V_L = -\frac{q}{\mu}\boldsymbol{A}(t)\cdot\hat{\boldsymbol{p}} + \frac{q^2A^2(t)}{2\mu}, \tag{S4}$$

where $q = e/2$ is the effective charge in relative motion and $\boldsymbol{A}(t)$ is the vector potential. Since the light considered here is very intense, the $A^2$ term in the interaction cannot be neglected as for weak light fields. And we show in the main text that this term plays an important role in the angular distributions of two-photon and three-photon absorptions. Also we are mainly interested in light with photon energies below the dissociation threshold (2.22 MeV), or the wavelengths being longer than about 550 fm, which is much larger than the size of the deuteron itself ($\approx$ 1 fm). The spatial variation of the vector potential can therefore be neglected. Here we choose $\boldsymbol{A}(t) = \boldsymbol{\epsilon}A_0\cos\omega t$, where the vector potential has been assumed to have a sinusoidal form linearly polarized along direction $\boldsymbol{\epsilon}$.

If at time $t_0$ the deuteron is in its ground state $|\psi_i\rangle$, then the probability amplitude of finding the system later in a final plane-wave state $|\psi_{\boldsymbol{p}}\rangle$ is

$$M_{\boldsymbol{p}}(t,t_0) = \langle\psi_{\boldsymbol{p}}|U(t,t_0)|\psi_i\rangle, \tag{S5}$$

with $\langle\boldsymbol{r}|\psi_{\boldsymbol{p}}\rangle = (2\pi)^{-3/2}e^{i\boldsymbol{p}\cdot\boldsymbol{r}}$. $U(t,t_0)$ is the time-evolution operator corresponding to the total Hamiltonian $H$. Because of the complexity of $V_{pn}$, there is no simple analytical form for $U(t,t_0)$. However, the time-evolution operators corresponding to the Hamiltonian $H_0$ and $H_L$ are much simpler with the following forms

$$U_0(t,t_0)|\psi_i\rangle = \exp\left\{-iE_i(t-t_0)\right\}|\psi_i\rangle; \tag{S6}$$

$$U_L(t,t_0)|\psi_{\boldsymbol{p}}\rangle = \exp\Big\{-i\big(\frac{p^2}{2\mu}+\eta\omega\big)(t-t_0) + i\sqrt{\eta\alpha}(\sin\omega t - \sin\omega t_0) - \frac{i\eta}{2}(\sin 2\omega t - \sin 2\omega t_0)\Big\}|\psi_{\boldsymbol{p}}\rangle. \tag{S7}$$

*Electronic address: xwang@gscaep.ac.cn

In Eq. (S6) $E_i$ is the energy of the ground state. In Eq. (S7) we have used Eqs. (S3, S4) and defined for convenience $\eta \equiv q^2 A_0^2/4\mu\omega$ and $\alpha = 4(\boldsymbol{\epsilon}\cdot\boldsymbol{p})^2/\mu\omega$. It is to be pointed out that $\eta\omega$ is the ponderomotive energy of the proton. Also the condition $\eta \ll 1$ holds for the parameters used in our calculation. This means that the ponderomotive energy is much smaller than the photon energy.

It can be proved that $U$ and $U_0$ are related by the following equation

$$U(t,t_0) = U_0(t,t_0) - i\int_{t_0}^{t} U(t,t_1)V_L(t_1)U_0(t_1,t_0)dt_1. \tag{S8}$$

## II. THE STRONG-FIELD APPROXIMATION

If the propagator $U$ inside the integral of Eq. (S8) is approximated by $U_L$, then the transition amplitude $M_{\boldsymbol{p}}$ in Eq. (S5) can be written as

$$M_{\boldsymbol{p}}(t,t_0) \;\approx\; -i\int_{t_0}^{t}\langle\psi_{\boldsymbol{p}}|U_L(t,t_1)V_L(t_1)U_0(t_1,t_0)|\psi_i\rangle dt_1. \tag{S9}$$

This approximation is called the strong-field approximation (SFA), developed by Keldysh [S1], Faisal [S2], and Reiss [S3]. The SFA transition amplitude has a clear physical picture: The system starts from the initial state $|\psi_i\rangle$ at $t_0$, propagates under the influence of $H_0$ until time $t_1$, when it is kicked by the laser potential $V_L$, and from $t_1$ to $t$ the system propagates under the influence of $H_L$, neglecting the effect of the the p-n binding potential. SFA has been widely used to describe the interaction between atoms and intense laser fields. In fact, as explained in the main text, SFA is more suitable for the deuteron system because the p-n potential is of short range, and neglecting the binding potential in the continuum state is more justified than for atoms with long-range Coulomb potentials.

We continue by substituting Eqs. (S4, S6, S7) into Eq. (S9). The following expansion will be used [S3]

$$\exp\left\{\frac{i\eta}{2}\sin 2\omega t - i\sqrt{\eta\alpha}\sin\omega t\right\} \approx \sum_{n=-\infty}^{\infty}\left(-\frac{\eta}{4}\right)^{n/2}\zeta_n(\alpha)e^{-in\omega t}, \quad \text{for} \quad \eta \ll 1 \tag{S10}$$

where $\zeta_n(\alpha) \equiv \sum_k (-\alpha)^k/(2k)!(n/2-k)!$, and $n$ takes integer values. For even $n$, $k = 0, 1, ..., n/2$; and for odd $n$, $k = 1/2, 3/2, ..., n/2$. The transition amplitude can then be written in the following concise form in the long-time limit (i.e., for pulses much longer than an optical period)

$$M_{\boldsymbol{p}}(t\to\infty, t_0\to-\infty) \approx i\frac{\tilde{\psi}_i(\boldsymbol{p})}{\sqrt{2\pi}}\sum_n n\omega\left(-\frac{\eta}{4}\right)^{n/2}\zeta_n(\alpha)\delta\left(\frac{p^2}{2\mu} - E_i - n\omega\right), \tag{S11}$$

where $\tilde{\psi}_i(\boldsymbol{p}) = (2\pi)^{3/2}\langle\psi_{\boldsymbol{p}}|\psi_i\rangle$ is a momentum component of the deuteron ground state. The transition amplitude is a summation over different disintegration channels, distinguished by the number of photons absorbed. For a channel with $n$ absorbed photons, the delta function imposes the energy conservation condition.

The differential rates (angular distributions) can be obtained by integrating out the final $\boldsymbol{p}$ in each solid angle

$$\begin{aligned}\frac{dw}{d\Omega} &= \int p^2 dp \lim_{\substack{t_0\to-\infty\\ t\to\infty}}\frac{|M_{\boldsymbol{p}}(t,t_0)|^2}{t-t_0}\\ &= \frac{\sqrt{2\mu^3\omega^5}}{4\pi^2}\sum_{n=n_0}^{\infty} n^2\sqrt{n+\frac{E_i}{\omega}}\left(\frac{\eta}{4}\right)^n|\tilde{\psi}_i(\boldsymbol{p}_n)|^2\zeta_n^2(\alpha_n)\end{aligned} \tag{S12}$$

where $n_0$ is the minimum number of photons required for dissociation (the integer just greater than $-E_i/\omega$) and $p_n = \sqrt{2\mu(E_i + n\omega)}$ fulfilling the delta-function energy constraint in Eq. (S11). The total disintegration rate can be obtained by integrating the differential rates over all solid angles.

As mentioned earlier the condition $\eta \ll 1$ holds in our calculation, and Eq. (S12) is a sum of $\eta^n$, only the $n_0$ term needs to be kept (That is, "above-threshold" disintegrations can be neglected). $n_0 = 1$ corresponds to single-photon disintegration which has been studied in traditional nuclear physics. $n_0 > 1$ corresponds to the cases that multiple photons need to be absorbed simultaneously to disintegrate the deuteron. Then the angular distribution Eq. (S12)

can be simplified to

$$\frac{dw}{d\Omega} \approx \frac{\sqrt{2\mu^3\omega^5}}{4\pi^2} n_0^2 \sqrt{n_0 + \frac{E_i}{\omega}} \left(\frac{\eta}{4}\right)^{n_0} |\tilde{\psi}_i(\boldsymbol{p}_{n_0})|^2 \sum_{k=0}^{n_0/2} \sum_{l=0}^{n_0/2} \frac{(-8)^{k+l} \left(n_0 + \frac{E_i}{\omega}\right)^{k+l} (\cos\theta)^{2k+2l}}{(2k)!\,(2l)!\,\left(\frac{n_0}{2} - k\right)!\,\left(\frac{n_0}{2} - l\right)!} \tag{S13}$$

for even $n_0$, and

$$\frac{dw}{d\Omega} \approx \frac{2\sqrt{2\mu^3\omega^5}}{\pi^2} n_0^2 \left(n_0 + \frac{E_i}{\omega}\right)^{\frac{3}{2}} \left(\frac{\eta}{4}\right)^{n_0} |\tilde{\psi}_i(\boldsymbol{p}_{n_0})|^2 \sum_{k=0}^{\frac{n_0-1}{2}} \sum_{l=0}^{\frac{n_0-1}{2}} \frac{(-8)^{k+l} \left(n_0 + \frac{E_i}{\omega}\right)^{k+l} (\cos\theta)^{2k+2l+2}}{(2k+1)!\,(2l+1)!\,\left(\frac{n_0-1}{2} - k\right)!\,\left(\frac{n_0-1}{2} - l\right)!} \tag{S14}$$

for odd $n_0$. Here $\theta$ is the polar angle with respect to $\boldsymbol{\epsilon}$, the direction of the laser vector potential.

It's easy to find that the kinetic energy of the center of mass $p_{\rm cm} \sim A_0^2/M$ is less than the photon energy $\omega$ by more than 10 orders of magnitude. Therefore the motion of the center of mass can be neglected. The kinetic energy of the emitted proton is less than the photon energy $\omega$ (neglecting above-threshold disintegrations). The momentum of the proton is therefore less than $\sqrt{2\mu\omega}$. With this condition the D-component of the deuteron ground state, constituting a few percent in population, contributes little to the disintegration. This is because the S-component has more low-momentum fractions than the D-component does. We have checked that the relative contribution from the D-component is less than $10^{-3}$ in the disintegration process.

For circularly polarized light, the vector potential can be described by

$$\boldsymbol{A}(t) = \frac{A_0}{2}\left(\boldsymbol{\epsilon} e^{i\omega t} + \boldsymbol{\epsilon}^* e^{-i\omega t}\right), \tag{S15}$$

where $\boldsymbol{\epsilon}\cdot\boldsymbol{\epsilon} = 0$, $\boldsymbol{\epsilon}\cdot\boldsymbol{\epsilon}^* = 1$. The differential disintegration rate reads

$$\frac{dw}{d\Omega} \approx \frac{\sqrt{2\mu^3\omega^5}}{4\pi^2} \frac{(n_0 + \frac{E_i}{\omega})^{n_0+\frac{1}{2}}}{[(n_0-1)!]^2} |\tilde{\psi}_i(\boldsymbol{p}_{n_0})|^2 \eta^{n_0} \left(\sin\theta\right)^{2n_0}. \tag{S16}$$

Only the $n_0$ order is kept. Note that for circular polarization, the polar angle $\theta$ is defined with respect to the laser propagation direction. One finds that the differential cross section depends on $\theta$ only through the last $(\sin\theta)^{2n_0}$ term. That is, for the same $n_0$, different photon energies lead to the same shape of angular distribution.

[S1] L. V. Keldysh, Sov. Phys. JETP **20**, 1307 (1965).
[S2] F. H. M. Faisal, J. Phys. B **6**, L89 (1973).
[S3] H. R. Reiss, Phys. Rev. A **22**, 1786 (1980).
